# Supplementary material for: Radiative cooling of a superconducting resonator
Source: arXiv:1910.01203 ancillary file (2019-10-02)
Supplement: Supplementary file 1 [file microwave_mode_ground_state_cooling_SUPPLEMENTAL.pdf]

# Supplemental Materials for "Radiative cooling of a superconducting resonator"

## I. RADIATIVE COOLING MODEL

Consider a mode of a superconducting resonator with an intrinsic damping rate $\kappa_{\rm i}$ and an external coupling rate $\kappa_{\rm e}$. Its equation of motion reads

$$\dot{\hat{a}}(t) = -\frac{\kappa}{2}\hat{a} - i\omega_0\hat{a} + \sqrt{\kappa_{\rm i}}\hat{a}_{\rm en} + \sqrt{\kappa_{\rm e}}\hat{a}_{\rm in}, \tag{S1}$$

where $\hat{a}$ is the annihilation operator of the mode, $\kappa = \kappa_{\rm i} + \kappa_{\rm e}$ is the total decay rate, $\omega_0$ is the the resonant frequency, and $\hat{a}_{\rm en}$ as well as $\hat{a}_{\rm in}$ are annihilation operators of the input field from the environment and the external coupling port, respectively. Fourier transforming Eq. (S1) to the frequency domain, we obtain

$$\hat{a}(\omega) = \frac{\sqrt{\kappa_{\rm i}}\hat{a}_{\rm en} + \sqrt{\kappa_{\rm e}}\hat{a}_{\rm in}}{\kappa/2 - i\Delta}, \tag{S2}$$

where $\Delta = \omega - \omega_0$.

Auto-correlations of the thermal input fields are

$$\langle \hat{a}^{\dagger}_{\rm en}(\omega)\hat{a}_{\rm en}(\omega')\rangle = \bar{n}_{\rm en}\delta(\omega - \omega'), \tag{S3}$$

$$\langle \hat{a}^{\dagger}_{\rm in}(\omega)\hat{a}_{\rm in}(\omega')\rangle = \bar{n}_{\rm in}\delta(\omega - \omega'), \tag{S4}$$

where $\bar{n}_{\rm en}$ and $\bar{n}_{\rm in}$ are thermal occupancies of the resonator's physical environment and the external bath respectively. Then the thermalized mode occupancy $\bar{n}_{\rm mode}$ can be found as

$$\bar{n}_{\rm mode} = \langle \hat{a}^{\dagger}(t)\hat{a}(t)\rangle = \frac{\kappa_{\rm i}\bar{n}_{\rm en} + \kappa_{\rm e}\bar{n}_{\rm in}}{\kappa_{\rm i} + \kappa_{\rm e}}, \tag{S5}$$

TABLE I. Symbol definitions.

| symbol | definition |
|---|---|
| $\hat{a}$ | annihilation operator of a superconducting resonator mode |
| $\hat{a}_{\rm en}$ | annihilation operator of field of the resonator's environment |
| $\hat{a}_{\rm in}$ | annihilation operator of ingoing field to the resonator through the external coupling port |
| $\hat{a}_{\rm out}$ | annihilation operator of outgoing field from the resonator |
| $\bar{n}_{\rm mode}$ | thermal occupancy of the resonator |
| $\bar{n}_{\rm in}$ | thermal occupancy of the external bath |
| $\bar{n}_{\rm en}$ | thermal occupancy of the environment |
| $S_{aa}$ | Spectral density of intracavity mode amplitude |
| $\bar{S}_{\rm in}$ | $\bar{S}a_{\rm in}a_{\rm in}$, symmetrized spectral density of ingoing field to the resonator |
| $\bar{S}_{\rm en}$ | $\bar{S}a_{\rm en}a_{\rm en}$, symmetrized spectral density of ingoing field to the resonator through the external coupling port |
| $\bar{S}_{\rm out}$ | $\bar{S}a_{\rm out}a_{\rm out}$, symmetrized spectral density of outgoing field from the resonator |
| $\bar{S}_{\rm out,off}$ | $\bar{S}_{\rm out}$ when the resonance is far detuned from the frequency window of interest |
| $\omega_0$ | superconducting resonator resonant frequency |
| $\kappa_{\rm i}$ | intrinsic coupling rate of the resonator |
| $\kappa_{\rm e}$ | external coupling rate of the resonator |
| $\mathcal{R}(\omega)$ | reflection spectrum of the resonator |
| $\mathcal{T}(\omega)$ | transmission spectrum for power coupled from the environment to the microwave circuit through the resonator |
| $\lambda$ | transmission of the transmission link connecting the thermal source and the resonator |
| $\bar{n}_{\rm eff,link}$ | effective environment temperature of the transmission link connecting the thermal source and the resonator |
| $G_0(\omega)$ | gain of the output line starting from the resonator |
| $N_{\rm add}(\omega)$ | added noise of the output line starting from the resonator |
| $G_{\rm s}(\omega)$ | gain of the output line starting from the output of the thermal source |

which aligns with the result obtained from detailed balance.

Given the definition of the spectral density of a variable $\hat{A}$

$$S_{AA}(\omega) = \int_{-\infty}^{\infty} d\tau e^{i\omega\tau} \langle \hat{A}^\dagger(0)\hat{A}(\tau)\rangle, \tag{S6}$$

the spectral density of the mode amplitude $\hat{a}$ can be found

$$S_{aa}(\omega) = \frac{\kappa_\mathrm{i}\bar{n}_\mathrm{en} + \kappa_\mathrm{e}\bar{n}_\mathrm{in}}{(\kappa/2)^2 + \Delta^2}, \tag{S7}$$

which is plotted in the Fig. 2(a) in the main text.

To analyze travelling noise power spectrum, we define symmetrized spectral density $\bar{S}_{AA}$ [S1] of a variable $\hat{A}$ as

$$\bar{S}_{AA}(\omega) = \big(S_{AA}(\omega) + S_{AA}(-\omega)\big)/2. \tag{S8}$$

For the output field, according to the input-output relation $\hat{a}_\mathrm{out} = -\hat{a}_\mathrm{in} + \sqrt{\kappa_\mathrm{e}}\hat{a}$, we find

$$\hat{a}_\mathrm{out}(\omega) = \frac{(\kappa_\mathrm{e} - \kappa_\mathrm{i})/2 + i\Delta}{\kappa/2 - i\Delta}\hat{a}_\mathrm{in} + \frac{\sqrt{\kappa_\mathrm{i}\kappa_\mathrm{e}}}{\kappa/2 - i\Delta}\hat{a}_\mathrm{en}, \tag{S9}$$

then the corresponding power spectral density is

$$\bar{S}_\mathrm{out}(\omega) = \mathcal{R}(\omega)\bar{n}_\mathrm{in} + \mathcal{T}(\omega)\bar{n}_\mathrm{en} + \frac{1}{2}, \tag{S10}$$

where

$$\mathcal{R}(\omega) = 1 - \kappa_\mathrm{i}\kappa_\mathrm{e}/\big((\kappa/2)^2 + (\omega - \omega_0)^2\big), \tag{S11}$$

$$\mathcal{T}(\omega) = \kappa_\mathrm{i}\kappa_\mathrm{e}/\big((\kappa/2)^2 + (\omega - \omega_0)^2\big). \tag{S12}$$

## II. FULL EXPERIMENTAL SETUP

Figure S1 shows a diagram of the full experimental setup. A superconducting resonator is mounted on VTS2 on the still plate of a dilution refrigerator. On the input line to the resonator, a 30 dB attenuator is mounted on VTS1 at temperature $T_\mathrm{s}$ in the mixing chamber. When the vector network analyzer (VNA) is not activated, the output of the 30 dB attenuator is predominately contributed by the Johnson-Nyquist noise at attenuator's temperature $T_\mathrm{s}$. Because the feed-through noise is suppressed by a factor of 1000, it is much smaller than the Johnson-Nyquist noise of the attenuator. Therefore, the 30 dB attenuator serves as a controllable thermal source. For simplicity, in the main text the 30 dB attenuator is treated as a matched load with no input.

Heaters and calibrated temperature sensors—ruthenium oxide temperature sensors for VTS1, and Cernox for VTS2—are mounted on both VTSs so that we can control and monitor their temperatures. By sending constant currents to the heaters, VTS1's temperature can be varied within a range from 70 mK to 1.5 K, while the VTS2's temperature can be varied between 1.02 K and 1.7 K. Within these ranges, the impact on the rest of the circuit is negligible.

One additional isolator is inserted between two circulators to enhance the isolation to suppress the resonance between the device and the amplifier. Superconducting NbTi coaxial cables (marked as golden color in the diagram) are used to connect components of different temperatures for low loss transmission as well as thermal isolation.

The output line starts with a Josephson parametric converter (JPC) operated as a phase preserving parametric amplifier followed by a high-electron-mobility transistor (HEMT) amplifier to provide low-noise amplification for detecting the output noise from the resonator.

## III. VARIABLE TEMPERATURE STAGES

The VTSs are key components in the experimental setup, as they provide independently variable temperatures $T_\mathrm{en}$ and $T_\mathrm{s}$, to enable noise thermometry calibration and radiative temperature control demonstration.

Both VTSs are designed to meet two requirements: (1) When the temperature varies, the rest of the circuits must not experience a significant temperature change; (2) The temperature gradient on each VTS must be minimized.

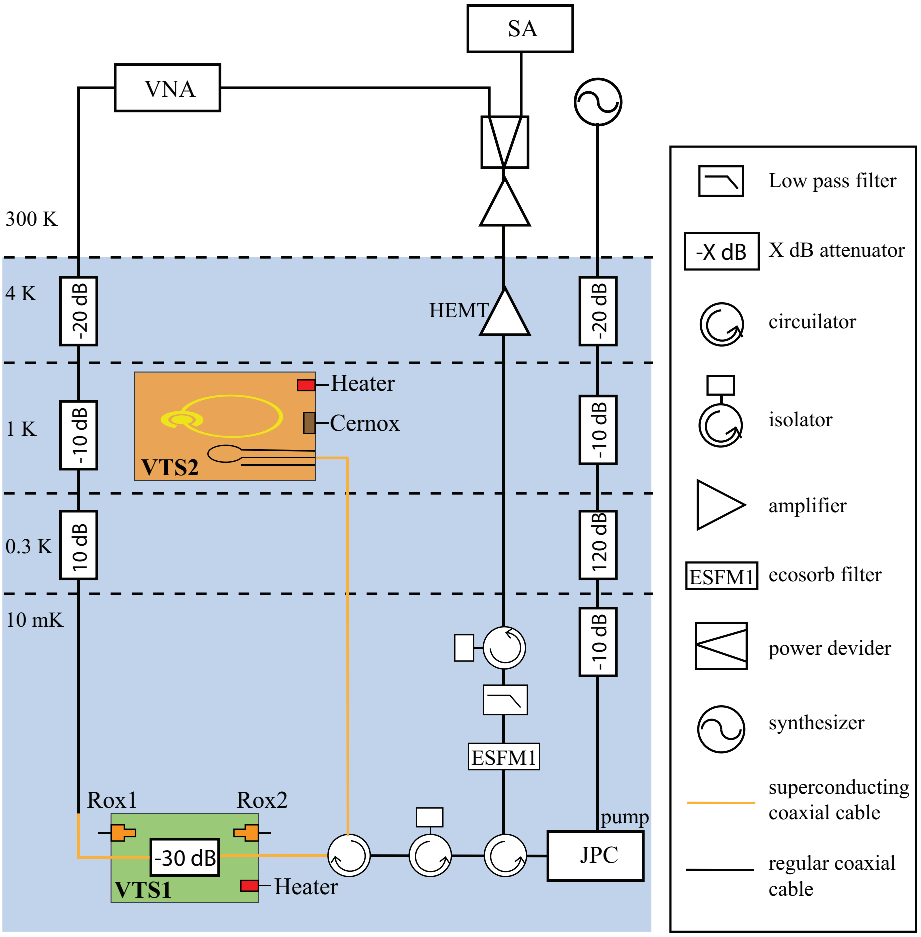


FIG. S1. Full experimental setup. For room temperature electronics, a vector network analyzer (VNA) is used to probe the superconducting resonance, and a spectrum analyzer (SA) is used for noise spectroscopic measurement. In the dilution fridge, two variable temperature stages (VTS) are mounted on the still plate and the mixing chamber respectively. Temperature sensors and a heater are installed on each VTS. Rox stands for ruthium oxide thermometer. A Josephson parametric converter in the output line (JPC) works as a phase-preserving parametric amplifier. Golden lines represent superconducting coaxial cables.

The former is realized by connecting each VTS to the fridge through a weak thermal link consisting of a 1-inch-long stainless steel post. Test results show a temperature rise less than 1 mK for the still plate when VTS2 is heated from 1 K to 2 K, and when VTS1 is heated from 70 mK to 1.5 K, the MXC's temperature rises from 17 mK to 50 mK, which results in negligible changes in thermal occupancies. The second requirement is important to ensure an accurate temperature readout through the temperature sensors mounted on the VTSs. To minimize the temperature gradients, the body of each VTS is made from oxygen-free copper, on which the heater and the attenuator (for VTS1) are held tightly in the middle with the gap filled with silicone grease. For VTS1, two ruthenium oxide temperature sensors are mounted on both sides of the stage. To monitor the temperature gradients, we recorded results given by both temperature sensors when VTS1 is slowly heated from 70 mK to 1.5 K. Results are shown in Fig. S2, where $x$-axis and $y$-axis represent temperatures read from each temperature sensor respectively. It is found that the both temperatures align perfectly to the specified temperature sensing accuracy .

## IV. JOSEPHSON PARAMETRIC CONVERTER ADDED NOISE CALIBRATION

The verification of radiative cooling requires a low-noise amplification chain that can confidently resolve noise spectral features at sub-quantum level. Hence a quantum-limited Josephson parametric converter (JPC) is employed as a pre-amplifier to provide low-noise amplification. The JPC has two resonances, named as the signal mode and the idler mode respectively, each resonating at around 10.5 GHz and 7.5 GHz respectively with more than 200 MHz

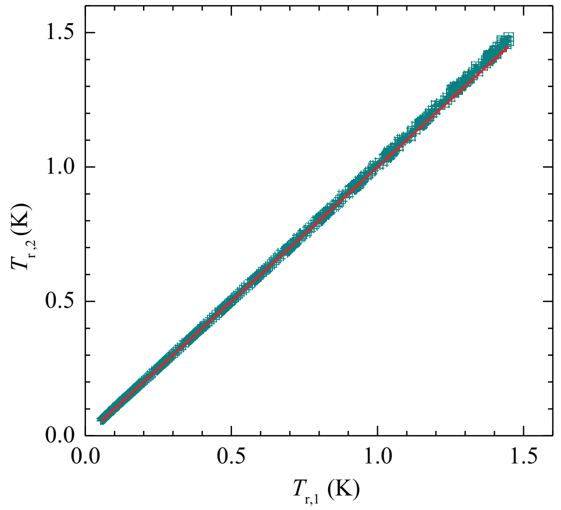


FIG. S2. Comparison between temperatures sensed by two temperature sensors mounted on two sides of VTS1, error bars corresponding to the sensing accuracy are plotted on each data points. The red trace represents the ideal case when $T_{\mathrm{r},1} = T_{\mathrm{r},2}$.

tunability. In this work, the JPC is powered by a pump at the sum of the signal and idler mode frequencies, to operate as a phase-preserving parametric amplifier for signals at the signal mode frequencies.

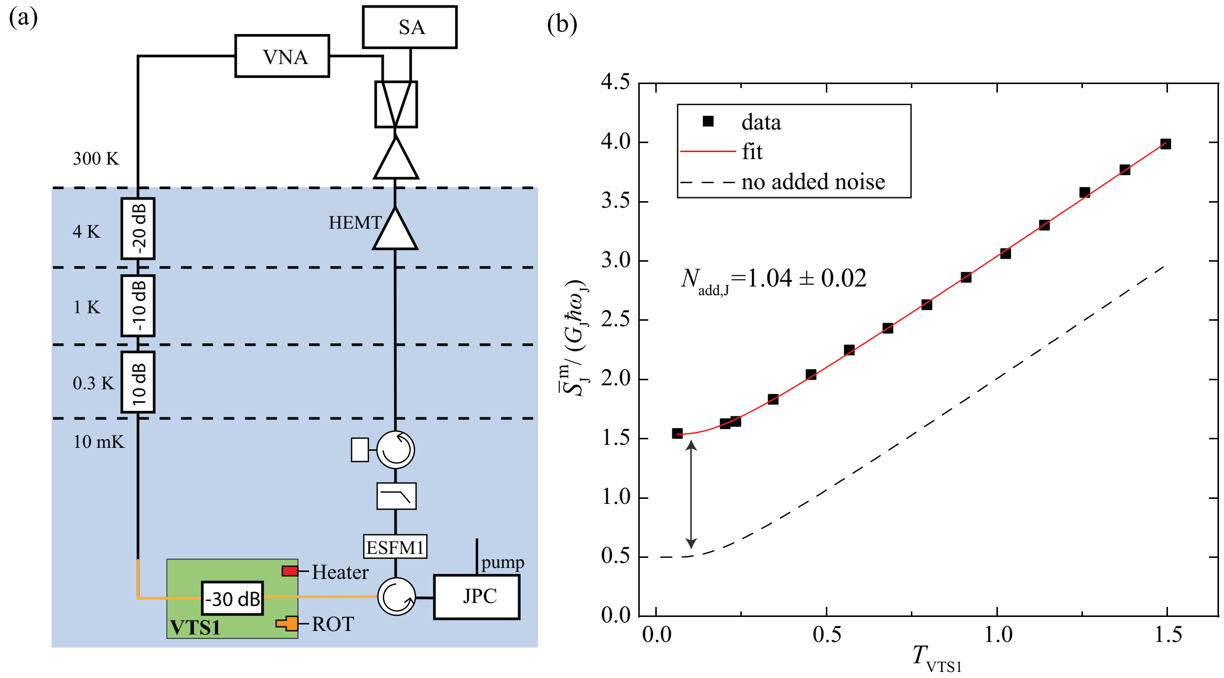


FIG. S3. Independent characterization of the output line featuring JPC as a pre-amplifier with setup shown in (a) and characterization results in (b). Plotted in (b) are measured power spectral density normalized to units of quanta as a function of the VTS1's temperature. During this calibration, the JPC's amplification is centered at 10.53 GHz with 27 dB gain to achieve minimized added noise.

In this section we show an independent characterization of an output line featuring the JPC in a separate experiment. The characterization setup is depicted in Fig. S3(a). A controllable thermal noise power is generated by the 30 dB attenuator mounted on the VTS before being amplified by the output line. The corresponding symmetrized power spectral density in units of quanta at the output of the attenuator is $S = \frac{1}{\exp(\mathrm{h}f/k_{\mathrm{B}}T_{\mathrm{VTS1}})-1} + \frac{1}{2}$. After going through

the output line, the expected measured power spectral density is

$$\bar{S}_{\rm J}^{\rm m} = G_{\rm J}\hbar\omega_{\rm J}\left(\frac{1}{\exp({\rm h}f/k_{\rm B}T_{\rm VTS1})-1}+\frac{1}{2}+N_{\rm add,J}\right), \tag{S13}$$

where $G_{\rm J}$ and $N_{\rm add,J}$ are the gain and added noise of the output line referred to the output of the 30 dB attenuator. The calibration is conducted at the frequency of $f = 2\pi\omega_{\rm J} = 10.53$ GHz. To ensure the output line is operated at the lowest added noise, JPC is pumped to generate a 27 dB gain at 10.53 GHz, such that the added noise is minimized.

Characterization results and a theoretical fit are shown in Fig. S3(b), where normalized $\bar{S}_{\rm J}^{\rm m}$ is plotted as a function of $T_{\rm VTS1}$. The fit to theoretical expression Eq. (S13) (red trace) reveals the $N_{\rm add,J}$ and $G_{\rm J}$ of the output line. Compared to the theoretical curve when no added noise (dashed line), the measured curve is elevated by the level of $N_{\rm add,J}$, which is found to be $1.04 \pm 0.02$ quanta. Thus the JPC is confirmed to be working at close to the quantum limit which produces 0.54 quanta excess noise.

## V. SUPERCONDUCTING RESONATOR FABRICATION, OPERATION AND CHARACTERIZATION

The design and more detailed discussion about the superconducting resonator are provided in Ref. [S2]. On the resonator, hole structures are patterned in the inductor wire, as shown in Fig. S4(a). By applying a perpendicular external magnetic field, the kinetic inductance can be modified by the induced screening supercurrent circulating the holes, thus the resonant frequency can be shifted.

The device is fabricated from a 50-nm-thick niobium nitride (NbN) film deposited on a sapphire substrate via atomic layer deposition. The pattern is defined by one single ebeam lithography step using hydrogen silsesquioxane (HSQ) resist, followed by chlorine dry etching. The remaining HSQ mask is removed using diluted buffered oxide etch.

To characterize the superconducting resonator, a weak coherent probe tone is sent to the resonator and then the reflection is measured by the VNA. The coherent tone is tailored to be very weak, corresponding to about 3 photons excited in the resonator, so that it does not saturate the two-level systems [S3–S5] and thereby modifying the coupling rates. As shown in Fig. S4, by fitting the reflection results (blue traces) to the theoretical model (black traces), coupling rates can be found.

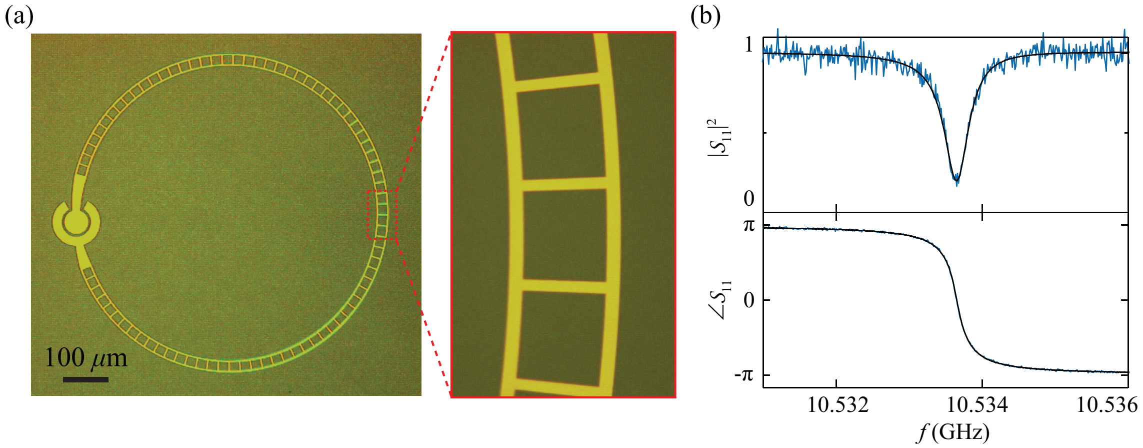


FIG. S4. (a) Optical image of the frequency-tunable superconducting resonator, insets shows the inductor wire where holes are patterned on. (b) Reflection spectrum of the resonator measured at 1.02 K with 0.7-mT bias magnetic field.

During the measurement, a 42.5-mA DC bias current was supplied to a superconducting coil to generate approximately 0.7 mT field to tune the resonant frequency to 10.5337 GHz. When the device is physically thermalized at 1.02 K, it is found $\kappa_{\rm i} = (113 \pm 1)$ kHz and $\kappa_{\rm e} = (298 \pm 2)$ kHz. By increasing the bias current to 43 mA, the resonance can be detuned by more than 15 MHz or 37 line-widths from 10.5337 GHz.

As resonator's physical temperature varies from 1 K to 1.45 K, it is found that the resonant frequency as well as $\kappa_{\rm i}$ slightly change accordingly. The variation of $\kappa_{\rm i}$ is less than 4% while $\kappa_{\rm e}$ remains constant. After the environment temperature increase beyond 1.5 K the intrinsic Q drops abruptly due to the degradation of superconductivity. For such a reason, in this experiment VTS2 only works within the range between 1 K and 1.45 K, and $\kappa_{\rm i}$ at each temperature is measured.

## VI. SYSTEM CALIBRATION

Output line noise thermometry calibration is conducted for a 5-MHz window centered at the JPC's peak amplification frequency. During the measurement, there are two types of spectra being meausured, $\bar{S}^{\mathrm{m}}_{\mathrm{out}}(\omega)$ and $\bar{S}^{\mathrm{m}}_{\mathrm{out,off}}(\omega)$. $\bar{S}^{\mathrm{m}}_{\mathrm{out}}(\omega)$ is the measured noise power spectral density spectrum when the resonator's resonant frequency is within the measurement frequency window, and $\bar{S}^{\mathrm{m}}_{\mathrm{out,off}}$ is the measured noise spectrum when the resonator's resonant frequency is detuned from the measurement window by increasing the external DC magnetic field. Based on the model, we have

$$\bar{S}^{\mathrm{m}}_{\mathrm{out}}(\omega) = G_0(\omega)\hbar\omega_0\left(\mathcal{T}(\omega)\bar{n}_{\mathrm{en}} + \mathcal{R}(\omega)\bar{n}_{\mathrm{in}} + \frac{1}{2} + N_{\mathrm{add}}(\omega)\right) \tag{S14}$$

$$\bar{S}^{\mathrm{m}}_{\mathrm{out,off}}(\omega) = G_0(\omega)\hbar\omega_0\left(\bar{n}_{\mathrm{in}} + \frac{1}{2} + N_{\mathrm{add}}(\omega)\right) \tag{S15}$$

$$\bar{n}_{\mathrm{in}} = \lambda\bar{n}_{\mathrm{s}} + (1-\lambda)\bar{n}_{\mathrm{eff,link}}, \tag{S16}$$

where $G_0(\omega)$ and $N_{\mathrm{add}}(\omega)$ represent the gain and added noise of the output line for the outgoing power from the resonator, they are both frequency dependent because of the limited bandwidth of JPC's amplification. $\bar{n}_{\mathrm{s}}$ denotes photon number of the output from the controllable thermal source. $\lambda$ characterizes the transmission of the transmission link between the controllable thermal source and the resonator, and $\bar{n}_{\mathrm{eff,link}}$ characterizes the effective thermal photon number coupled into the transmission link through the loss. When the resonance is detuned, $\mathcal{R}(\infty) = 1$ and $\mathcal{T}(\infty) = 0$, so Eq. (S14) reduces to Eq. (S15).

Because $G_0(\omega)$, $N_{\mathrm{add}}(\omega)$, $\lambda$ and $\bar{S}_{\mathrm{eff}}$ have or may have temperature dependence, both VTSs are made to have very weak thermal links the fridge, such that when $\bar{n}_{\mathrm{s}}$ and $\bar{n}_{\mathrm{en}}$ vary, these variables do not change accordingly. Slight JPC gain drift (less than 0.4 dB) is observed over hours of measurement and constantly monitored by the VNA, before being factored out from the measurement results, so it is safe to assume $G_0(\omega)$ and $N_{\mathrm{add}}(\omega)$ are both constant over time. By adopting Eq. (S14-S16), we assume no impedance mismatches at connectors, thereby no resonance anywhere in the circuit other than the superconducting resonator.

To start the system calibration, the first task is to find out the gain of the output line for the outgoing power from the 30 dB attenuator, denoted by $G_{\mathrm{s}}$, which has relation $G_{\mathrm{s}} = G_0\lambda$. To this end, we sweep the 30 dB attenuator's temperature, essentially $\bar{n}_{\mathrm{s}}$. At each temperature, the output spectrum $\bar{S}^{\mathrm{m}}_{\mathrm{out,off}}$ is measured. Combining Eqs. (S15) and (S16), $G_{\mathrm{s}}$ can be found as the dependence of $\bar{S}^{\mathrm{m}}_{\mathrm{out,off}}$ on $\bar{n}_{\mathrm{s}}$

$$G_{\mathrm{s}}(\omega) = \frac{1}{\hbar\omega_0}\frac{\partial\bar{S}^{\mathrm{m}}_{\mathrm{out,off}}}{\partial\bar{n}_{\mathrm{s}}}. \tag{S17}$$

Plotted in Fig. S5(a) are $\bar{S}^{\mathrm{m}}_{\mathrm{out,off}}$ as functions of $\bar{n}_{\mathrm{s}}$ at different frequencies. As Eq. (S17) suggested, the slope of each curve represents the gain $G_{\mathrm{s}}$ at a frequency. Complete $G_{\mathrm{s}}(\omega)$ results at different frequencies are plotted in Fig. S5(b), the frequency dependence reflects the gain profile of the JPC.

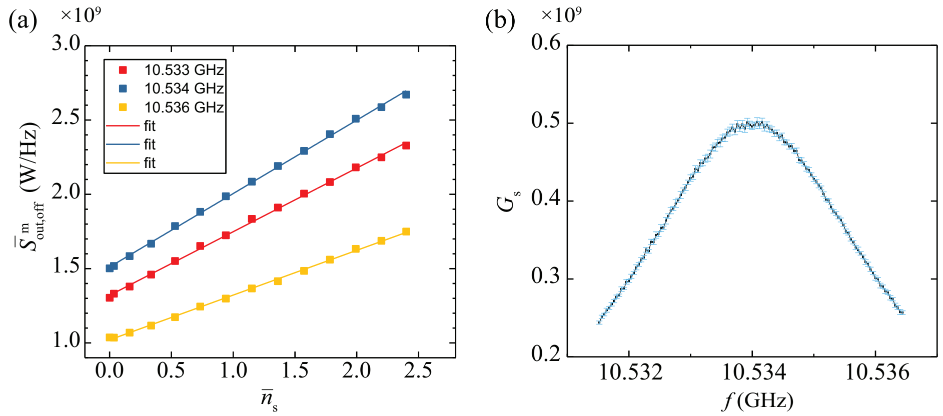


FIG. S5. Calibration to find $G_{\mathrm{s}}(\omega)$. During this measurement, the VTS2's temperature is fixed at 1.02 K, while the temperature of VTS1 is swept. (a) depicts the linear growth of $\bar{S}^{\mathrm{m}}_{\mathrm{out,off}}$ with increased $\bar{n}_{\mathrm{s}}$, in which the slope of each curve represents $G_{\mathrm{s}}(\omega)$ at the corresponding frequency. Results of $G_{\mathrm{s}}(\omega)$ over the full frequency range of interest in plotted in (b).

Then we find out the gain and added noise of the output line with the help of the known $G_{\mathrm{s}}(\omega)$. During this sets of measurements, the environment temperature of the resonator (VTS2) is swept, while VTS1's temperature is fixed

at 70 mK, resulting $\bar{n}_{\mathrm{s}} = 0.001$. At each temperature we measure the $\bar{S}^{\mathrm{m}}_{\mathrm{out}}$ and $\bar{S}^{\mathrm{m}}_{\mathrm{out,off}}$ spectrum. Define a difference spectrum $\Delta\bar{S}^{\mathrm{m}}_{\mathrm{out}} = \bar{S}^{\mathrm{m}}_{\mathrm{out}} - \bar{S}^{\mathrm{m}}_{\mathrm{out,off}}$, from Eq. (S14) and (S15), the theoretical expectation of $\Delta\bar{S}^{\mathrm{m}}_{\mathrm{out}}$ is expressed as

$$\Delta\bar{S}^{\mathrm{m}}_{\mathrm{out}}(\omega) = G_0(\omega)\hbar\omega_0\mathcal{T}(\omega)\big(\bar{n}_{\mathrm{en}} - \bar{n}_{\mathrm{in}}\big). \tag{S18}$$

Combining with the knowledge of $G_{\mathrm{s}}(\omega)$, we can eliminate the frequency dependence caused by the output line in the $\Delta\bar{S}^{\mathrm{m}}_{\mathrm{out}}$ curve,

$$\frac{\Delta\bar{S}^{\mathrm{m}}_{\mathrm{out}}}{G_{\mathrm{s}}\hbar\omega_0}(\omega) = \lambda\mathcal{T}(\omega)\big(\bar{n}_{\mathrm{en}} - \bar{n}_{\mathrm{in}}\big). \tag{S19}$$

Plotted in Fig. S6(a) are a set of $\frac{\Delta\bar{S}^{\mathrm{m}}_{\mathrm{out}}}{G_{\mathrm{s}}\hbar\omega_0}(\omega)$ spectral at different environment temperatures. Each curve exhibit a Lorentzian line shape, which fits perfectly to Eq. (S19) (solid curves), with coupling rates characterized by the VNA. When temperature rises, the amplitude of the peak grows accordingly. From each fit, we can extract $\lambda\Delta\bar{n}$ from a $\frac{\Delta\bar{S}^{\mathrm{m}}_{\mathrm{out}}}{G_{\mathrm{s}}\hbar\omega_0}(\omega)$ spectrum, where $\Delta\bar{n} \equiv \bar{n}_{\mathrm{en}} - \bar{n}_{\mathrm{in}}$. Acquired $\lambda\Delta\bar{n}$ are plotted as a function of the environment thermal occupancy $\bar{n}_{\mathrm{en}}$ in Fig. S6(b), where a linear relation is observed. Through a linear fitting, we can find $\lambda$ as the slope and $\bar{n}_{\mathrm{in}}$ as the intersect to the $x$-axis. Because during this measurement, the VTS1's temperature is fixed at 70 mK, corresponding to $\bar{n}_{\mathrm{s}} = 0.001$, thus $\bar{n}_{\mathrm{in}} \approx (1-\lambda)\bar{n}_{\mathrm{eff,link}}$. Calibration results are $\lambda = 0.91 \pm 0.04$ and $\bar{n}_{\mathrm{in}} \approx (1-\lambda)\bar{n}_{\mathrm{eff,link}} = 0.02^{+0.06}_{-0.02}$.

Moving on, $G_0(\omega)$ can be obtained as $G_0(\omega) = G_{\mathrm{s}}(\omega)/\lambda$. Once $G_0(\omega)$ is found, $N_{\mathrm{add}}(\omega)$ can be calculated based on Eq. (S15) and measured $\bar{S}^{\mathrm{m}}_{\mathrm{out,off}}$. $N_{\mathrm{add}}(\omega)$ is found to be between 2.7 and 3.2 quanta at different frequencies.

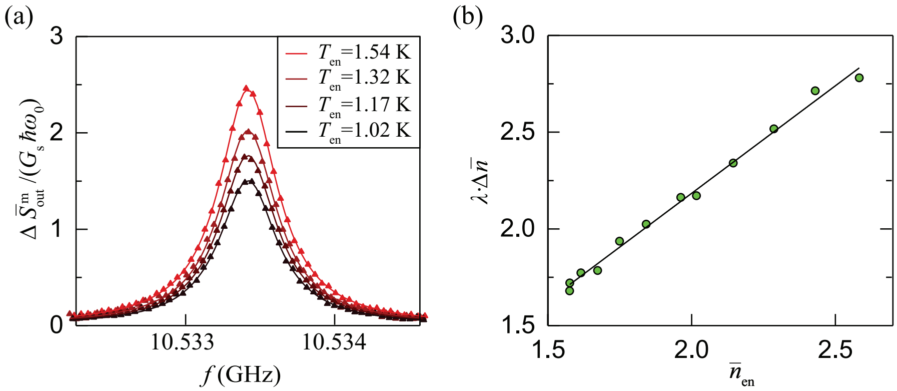


FIG. S6. Localized noise thermometry calibration. During this measurement, the VTS2's temperature is swept while the temperature of VTS1 is fixed at 0.07 K. (a) depicts the normalized output spectrum $\frac{\Delta\bar{S}^{\mathrm{m}}_{\mathrm{out}}}{G_{\mathrm{s}}\hbar\omega_0}(\omega)$ at different environment temperatures $T_{\mathrm{en}}$. Theoretical fits are shown as the solid curves. From the theoretical fit, obtained $\lambda\Delta\bar{n}$ are plotted against $\bar{n}_{\mathrm{en}}$ in (b), which exhibits a linear relation.

## VII. FANO RESONANCE INDUCED BY INTERFERENCE IN A MICROWAVE CIRCUIT

In Fig. 3, asymmetric line shape is observed in some of the output noise spectra, which are typically recognized as Fano resonances. A Fano resonance is usually caused by interference between two pathways, one of which being the reflection from the resonator. This phenomena have been observed and studied in a variety of systems consisting of coupled resonators, and is interchangeable with EIT-like resonance under some circumstances [S6].

In our system, the Fano resonance is a result of the interference owing to the imperfection of the circulator, which circuit model is shown in Fig. S7. For an ideal circulator, the transmission $3 \to 1$ is forbidden, while only transmission $1 \to 2$, $2 \to 3$ and $3 \to 1$ are allowed. However, in practice, a finite transmission $3 \to 1$ will cause interference between the pathways $1 \to 2 \to$ resonator $\to 2 \to 3$ and $1 \to 3$, thereby induces Fano resonance.

Before we get into more detailed discussion on the Fano resonance phenomenon, it is worth noting that Fano resonance is a secondary effect in our system. Because the circulator has an isolation greater than 24 dB, the Fano effect is well suppressed. As shown in Fig. S4(b) and Fig. S6(a), the reflection spectrum and output noise spectrum both fit the symmetric Lorentzian function very well. As a result, the resonator can be approximated to a regular non-Fano resonator to a good precision.

In this section, we are going to derive the Fano resonance from a circuitry model consisting of an imperfect circulator. To start with, we assume a symmetrical $\mathcal{S}$-matrix for the circulator,

$$\mathcal{S} = \begin{bmatrix} \beta & \gamma & t \\ t & \beta & \gamma \\ \gamma & t & \beta \end{bmatrix}, \quad \text{(S20)}$$

then the input and output field as marked in Fig. S7 satisfy relation

$$\begin{bmatrix} \hat{a}'_1 \\ \hat{a}'_2 \\ \hat{a}'_3 \end{bmatrix} = \mathcal{S} \begin{bmatrix} \hat{a}_1 \\ \hat{a}_2 \\ \hat{a}_3 \end{bmatrix}. \quad \text{(S21)}$$

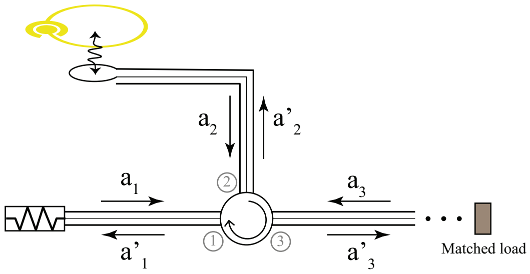


FIG. S7. A circuitry with imperfect circulator, Fano resonance is produced through the interference between the pathways $1 \to 2 \to$ resonator $\to 2 \to 3$ and $1 \to 3$.

Since port 2 of the circulator interfaces the resonator, the input to port 2 is constituted by the reflected wave and the transmitted wave from the environment

$$\hat{a}_2 = r_0 \hat{a}'_2 + t_0 \hat{a}_{\text{en}}, \quad \text{(S22)}$$

$$\langle \hat{a}^\dagger_{\text{en}}(t) \hat{a}_{\text{en}}(t') \rangle = \bar{n}_{\text{en}} \delta(t - t'), \quad \text{(S23)}$$

where $r_0 = \frac{(\kappa_{\text{i}} - \kappa_{\text{e}})/2 + i\Delta}{\kappa/2 - i\Delta} * e^{-i2\phi}$, and $t_0 = \frac{\sqrt{\kappa_{\text{i}}\kappa_{\text{e}}}}{\kappa/2 - i\Delta} * e^{-i\phi}$, see Eq. S9 for derivation. Here $\phi$ is the additional phase shift caused by the finite length of the transmission line between the circulator and the resonator. Without losing generality, we assume matched loads terminating port 1 and 3. So the input to port 1 and 3 are thermal radiations of the load, whose bath occupancy are denoted by $\bar{n}_{\text{s}}$ and $\bar{n}_3$ respectively. In the real experiment setup, port 3 is terminated by the pre-amplifier JPC, which temperature is below 70 mK by thermalizing to the mixing chamber, hence we assume $\bar{n}_3 = 0$. The input to port 1 and 3 can then be summarized as

$$\langle \hat{a}^\dagger_1(t) \hat{a}_1(t') \rangle = \bar{n}_{\text{s}} \delta(t - t'), \quad \text{(S24)}$$

$$\langle \hat{a}^\dagger_3(t) \hat{a}_3(t') \rangle = 0, \quad \text{(S25)}$$

In addition, for simplicity, the circuit is assumed to be placed in a very cold environment that all the noise coupled from the environment to the microwave circuit through the loss are vacuum noise.

Combining Eqs. (S20)-(S22), we can solve the output field $\hat{a}'_3$ to the first order,

$$\hat{a}'_3 = \frac{t t_0(\Delta) \hat{a}_{\text{en}} + (t^2 r_0(\Delta) + \beta) \hat{a}_1}{1 - \gamma r_0}. \quad \text{(S26)}$$

In the case of a perfect circulator, namely $\beta = 0$, $\gamma = 0$, and $t = 1$, then the output field will be reduced to

$$\hat{a}'_3 = t_0(\Delta) \hat{a}_{\text{en}} + r_0(\Delta) \hat{a}_1, \quad \text{(S27)}$$

which describes a perfect Lorentzian shaped spectrum.

Combining Eqs. (S23), (S24), and (S27), the output power spectrum can be calculated

$$\bar{S}_{a_3'a_3'} = \left|\frac{tt_0(\Delta)}{1-\gamma r_0}\right|^2 \bar{n}_{\rm en} + \left|\frac{t^2 r_0(\Delta)+\beta}{1-\gamma r_0}\right|^2 \bar{n}_{\rm s} + \frac{1}{2}. \tag{S28}$$

Following this equation, we compute output noise spectra by plugging in realistic parameters. For the circulator, we assigned $\beta = 0.04e^{i4.6\pi}$, $\gamma = 0.065e^{i0.52\pi}$, $t = 0.975$ and $\phi = 0.02\pi$, which correspond to an insertion loss of 0.4 dB, an isolation of -24 dB and a VSWR of 1.08, within the specified range. Furthermore, the environment temperature is assigned to be 1.02 K to match the condition when data in Fig. S8(a) is obtained. Shown in Fig. S8(b) are a set of output spectra $\bar{S}_{a_3a_3}$ computed with different $T_{\rm s}$, to simulate the change of thermal source temperature in the real experiment. In Fig. S8(b), similar asymmetric spectra to measurement results in Fig. S8(a) are reproduced, suggesting the interference induced by the imperfect circulator may be the origin of the Fano resonance.

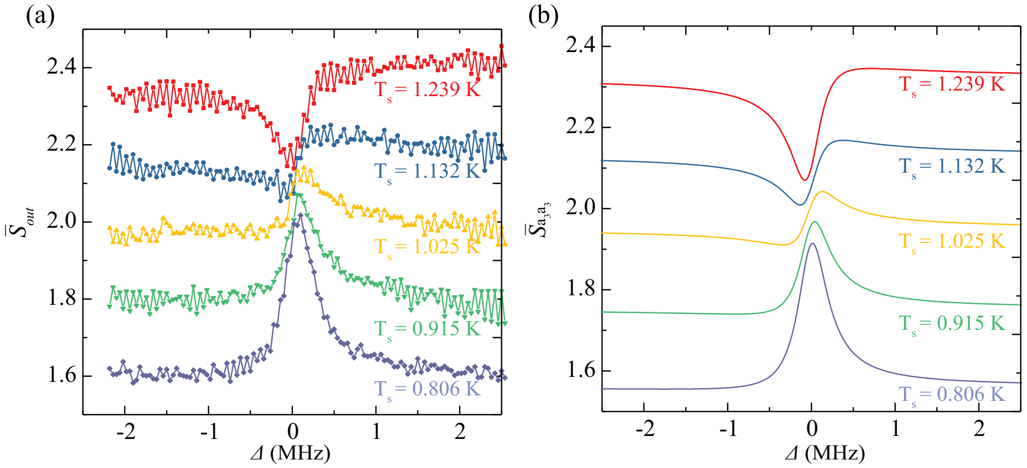


FIG. S8. (a) Measured $\bar{S}_{\rm out}$ noise spectrum when $T_{\rm en}$ is fixed at 1.02 K. (b) computed $\bar{S}_{a_3a_3}$ noise spectrum based on the circuitry model with $T_{\rm en}$ set to be 1.02 K. In both figures, the different traces correspond to different external thermal source temperatures $T_{\rm s}$.


[S1] A. A. Clerk, M. H. Devoret, S. M. Girvin, F. Marquardt, and R. J. Schoelkopf, Rev. Mod. Phys. **82**, 1155 (2010).

[S2] M. Xu, X. Han, W. Fu, C.-L. Zou, and H. X. Tang, Appl. Phys. Lett. **114**, 192601 (2019).

[S3] L. Faoro and L. B. Ioffe, Phys. Rev. Lett. **109**, 157005 (2012).

[S4] T. Lindström, J. E. Healey, M. S. Colclough, C. M. Muirhead, and A. Y. Tzalenchuk, Phys. Rev. B **80**, 132501 (2009).

[S5] P. Macha, S. H. W. van der Ploeg, G. Oelsner, E. Ilichev, H.-G. Meyer, S. Wnsch, and M. Siegel, Applied Physics Letters **96**, 062503 (2010), https://doi.org/10.1063/1.3309754.

[S6] B.-B. Li, Y.-F. Xiao, C.-L. Zou, Y.-C. Liu, X.-F. Jiang, Y.-L. Chen, Y. Li, and Q. Gong, Appl. Phys. Lett **98**, 021116 (2011).
